# Supplementary material for: Rules, Choice, and Chance: A Welfare Evaluation Framework for Student-School Matching
Source: arXiv:2611.11514 source file (2026-11-08)
Supplement: Supplementary file 1 [file additional_details_trace.tex]

\subsection{Additional details about \sys}
\label{app:trace}

\begin{figure}[ht!]
\centering
\includegraphics[width=\linewidth]{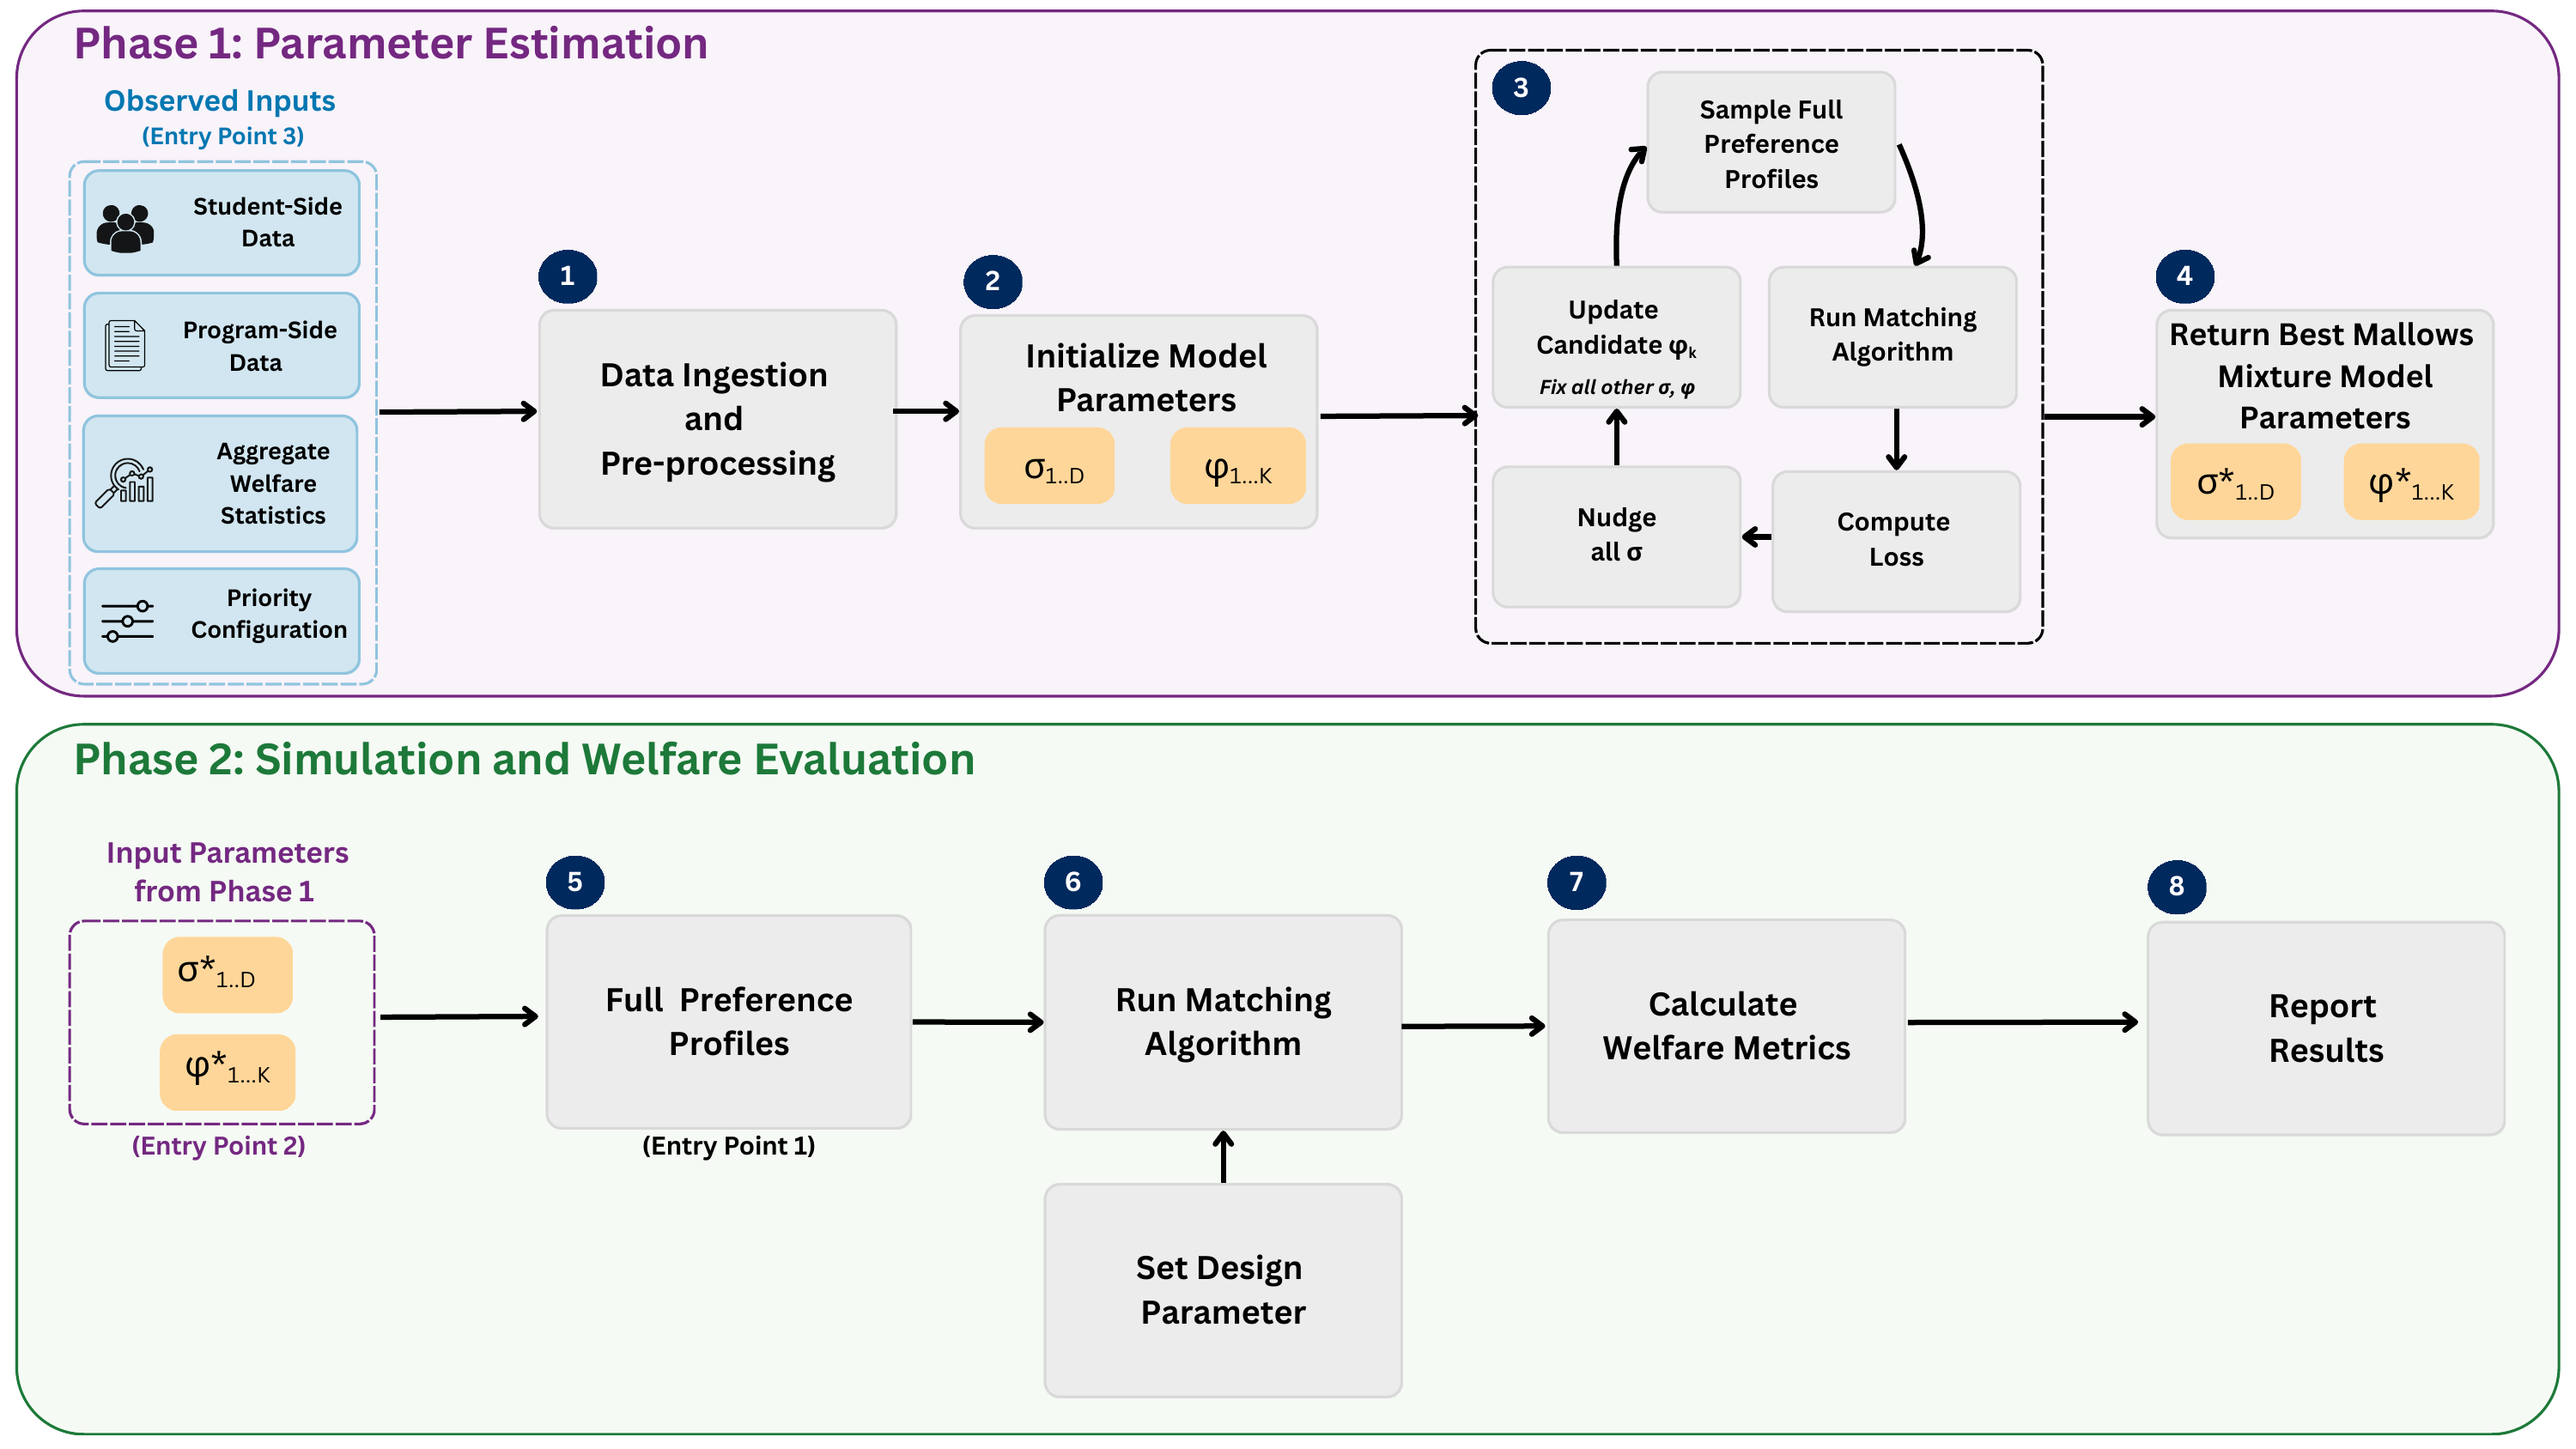}
\caption{Architecture of \sys (Trade-offs in Rules, Agency, Chance, and Equity).}
\label{fig:MAIarchitecture}
\end{figure}

Figure \ref{fig:MAIarchitecture} illustrates the workflow of our framework, \sys.
\sys offers three distinct entry points that determine how a user engages with the workflow in the first place. These entry points sit logically upstream of the inputs depicted: depending on which entry point a user adopts, a different subset of the observed inputs is required, and a different portion of the workflow is executed.

\textbf{Entry~point~3} (aggregate statistics only) requires four classes of input:

\begin{enumerate}
    \item \textbf{Student-side data.} 
    This includes the total number of applicants $|I|$, the applicant attribute profile $X = (x_i)_{i \in I}$ when available, and the
distribution of applicants across the subdivisions of interest
$\{I_d\}_{d \in \mathcal{D}}$ (e.g., residential districts in NYC,
regions in Chile).
These subdivisions define both the subgroups used for group-level
welfare analysis and the units at which central rankings are estimated.
The input may also include applicant attributes that feed into the
priority system, such as special priority statuses (e.g., Students with
Disabilities, sibling status), as well as the empirical distribution of
preference list lengths $L_i$ when available.

    \item \textbf{Program-side data.}
This includes program-level identifiers $\mathcal{J}$, seat capacities
$c_j$, the number of offers made by each program, and
admitted-student counts.
These quantities anchor the program side of the matching market and
allow the framework to compute simulated utilization $u_j(\mu)$ and
compare it against observed fill rates during the central-ranking
nudge step.

\item \textbf{Aggregate welfare statistics.}
The set of group-level outcome statistics against which the simulation
is calibrated.
For each subdivision $d \in \mathcal{D}$, this consists of an observed
(or, in a fully counterfactual exercise, a target) outcome vector built
from the welfare metrics defined in Section~\ref{prel}.
In the NYC case study ($v = 4$):
\[
    o_d \;=\; \bigl(
        W_3(\mu \mid d),\;
        W_5(\mu \mid d),\;
        W_{10}(\mu \mid d),\;
        W_{\mathrm{unmatch}}(\mu \mid d)
    \bigr).
\]
These statistics serve as the target moments in the Gaussian
log-likelihood objective (Eq.~\ref{eq:lik}), and they are the primary
signal from which the framework learns the dispersion and
central-ranking parameters.
Using subdivision-level targets ensures that the simulation is
calibrated to subgroup-specific outcomes rather than population-level
averages only.

\item \textbf{Priority configuration.}
A structured specification of the priority system governing admission
at each program.
This includes: the ordering of priority tiers (e.g., sibling priority,
district residence, academic screen); the partition of seats into
reserved pools and the corresponding reserve fractions (e.g., the
share of seats set aside for Students with Disabilities or
low-income applicants); and the admission-method classification where
applicable (e.g., unscreened, screened, EdOpt, or zoned in NYC).
Together these determine the reserve buckets $b_{ij}$, priority tiers
$t_{ij}$, and tie-breaking rules $\lambda_{ij}$ that enter the
composite priority score $\rho_{ij} = \alpha b_{ij} + \beta t_{ij} +
\lambda_{ij}$.
\end{enumerate}


\smallskip \textbf{Data Ingestion and Pre-Processing}

The pipeline ingests the inputs described above and produces three data
structures used throughout the estimation procedure.

\begin{enumerate}[label=(\roman*)]
    \item A \emph{program-level applicant matrix} containing
    subdivision-by-program counts of total applicants $A_{d,j}$ and
    true applicants $T_{d,j}$.
    \item A \emph{program-level information table} containing
    capacities $c_j$ and utilization estimates $u_j$.
    \item A \emph{subdivision-level statistics table} containing the
    observed aggregate outcome vectors $\{o_d\}_{d \in \mathcal{D}}$.
\end{enumerate}

Because NYC admissions data are reported at the program level,
the framework indexes choice objects by $j \in \mathcal{J}$ rather than
by schools $s \in \mathcal{S}$.
A program $j$ may be offered by a school $s$, but the estimation
procedure treats programs as the relevant matching objects and
capacities $c_j$ are defined at the program level accordingly.

\smallskip \textbf{Priority-Aware Matching}
%\label{app:priority}

To faithfully represent complex priority systems---including
multiple reserve pools, heterogeneous admission methods, and
intersecting eligibility categories---the framework expands each
program $j$ into a set of \emph{virtual programs}: one per seat pool
and admission sub-group, each carrying its own capacity.

Student priority attributes (e.g., residential borough, disability
status, academic performance, continuing-enrollment status) are sampled
from distributions calibrated to the priority configuration.
Each applicant's preference list $R_i$ is mapped to a ranked list over
virtual programs consistent with their sampled attributes, routing each
student to the virtual program corresponding to their seat pool and
sub-group eligibility.
Each student--virtual-program pair is then assigned a priority score
$\rho_{ij} = \alpha b_{ij} + \beta t_{ij} + \lambda_{ij}$ (with
$\alpha \gg \beta \gg 1$) from the reserve bucket $b_{ij}$, priority
tier $t_{ij}$, and lottery tie-breaker $\lambda_{ij}$.

The matching algorithm $M$ is run over virtual programs using
$\rho_{ij}$ as the program-side priority ordering; matches are then
mapped back to parent programs for welfare evaluation.
A single lottery permutation $\lambda$ is drawn once per EM round and
held fixed across all $N_{\mathrm{sim}}$ simulations and
$\phi$-evaluations within that round, reducing variance in the
stochastic objective without introducing systematic bias.
\\
\\
\textbf{List-Length Distribution}
%\label{app:listlength}

Submitted list lengths $L_i$ are drawn from one of two distributions,depending on data availability.
\\
\\
\textbf{Empirical distribution.}
When the full distribution of submitted list lengths is available in
the input data, list lengths are drawn directly from the empirical
distribution $\mathcal{L}(\theta_L)$.
This is the preferred option when working with real admissions records,
as it preserves the observed marginal distribution of $L_i$ exactly.
\\
\\
\textbf{Clipped Gaussian.}
When only summary statistics are available, list lengths are drawn from
a clipped Gaussian
$\mathcal{G}_{[L_{\min}, L_{\max}]}(m_L, s_L)$,
truncated to the interval $[L_{\min}, L_{\max}]$.
The mean $m_L$ can be inferred from the total number of applications
and the number of applicants; the standard deviation $s_L$ and clip
bounds $L_{\min}$, $L_{\max}$ are set based on available
administrative information or reasonable defaults (e.g., the maximum
ballot length permitted by the system).

In both cases, once $L_i$ is drawn, the full ranking
$\tau_i \sim \mathrm{Mallows}(\sigma_d, \phi_{k_i})$ produced by RIM
is truncated to its top $L_i$ entries to form the submitted preference
list $R_i$~\citep{Chakraborty2021}.
